# Supplementary material for: Distribution-aware Goal Prediction and Conformant Model-based Planning for Safe Autonomous Driving
Source: arXiv:2212.08729 source file (2022-12-16)
Supplement: Supplementary file 1 [file supplementary.tex]

\section{Network and Training Details}

During training, our experiments involve generating 39 steps, given a trajectory history of 20 steps. The trajectories are represented as 2D position sequences recorded at every 0.5 seconds. The hyperparameters of the network structure is described in Table~\ref{suppl:tab:hyperparameters}.

\begin{table*}[!h]
\caption{Network Hyperparameters.}
\label{suppl:tab:hyperparameters}
\begin{center}
\scriptsize
\begin{tabular}{l c l c l c l}
\toprule
Operation & & Input (dim.) & & Output (dim.) & & Parameters\\ 
\hline
\multicolumn{7}{c}{\textsc{ConvNet}} \\
\multicolumn{7}{c}{\text{(Every Conv2D is with `same' padding, and followed by BN \cite{ioffe2015batch} \& ReLU.)}} \\
\hline
\textit{Conv2D} & & $\bm{\Phi}~(64, 64, 3)$ & & \textit{conv}1~(64, 64, 16) & & kernel$\coloneqq$(3,3) \\
\textit{Conv2D} & & \textit{conv}1 & & \textit{conv}2~(64, 64, 16) & & kernel$\coloneqq$(3,3) \\
\textit{MaxPool2D} & & \textit{conv}2 & & \textit{pool}2~(32, 32, 16) & & kernel$\coloneqq$(2,2), stride$\coloneqq$(2,2) \\
\textit{Conv2D} & & \textit{pool}2 & & \textit{conv}3~(32, 32, 32) & & kernel$\coloneqq$(5,5) \\
\textit{Conv2D} & & \textit{conv}3 & & \textit{conv}4~(32, 32, 6) & & kernel$\coloneqq$(1,1) \\
\textit{Dropout} & & \textit{conv}3 & & $\bm{\Gamma}_{g}$~(32, 32, 32) & & p$\coloneqq$0.5 \\
\textit{UpSample2D} & & \textit{conv}4 & & $\bm{\Gamma}_{l}$~(100, 100, 6) & & mode$\coloneqq$bilinear \\
\hline
\multicolumn{7}{c}{\textsc{Trajectory Encoding Module}} \\
\multicolumn{7}{c}{(\text{Repeated for} $a \in \{1,2,...,A\}$ \text{with variable encoding time length} $T_{\textit{past}}^{a}\coloneqq t^{a}_{s}+1$)} \\
\hline
\textit{Difference} & & $S^{a}_{\textit{past}}~(T^{a}, 2)$ & & $\textit{dS}^{a}_{\textit{past}}~(T^{a}, 2)$ & & \text{zero-pad (at the \textit{start time}}) \\
\textit{Fully-connected} & & $\textit{dS}^{a}_{\textit{past}}$ & & $\textit{tS}^{a}_{t}~(T^{a}, 128)$  & & \text{activation}$\coloneqq$\text{Linear} \\
\textit{LSTM} & & $\textit{tS}^{a}_{t}$ & & $h^{a}_{0}~(128)$ & & \text{zero initial states} \\
\hline
\multicolumn{7}{c}{\textsc{Cross-agent Interaction Module}} \\
\multicolumn{7}{c}{$\text{(Repeated for } a \in \{1,2,...,A\})$} \\
\hline
\textit{LayerNorm} & & $\textit{h}^{a}_{0}~(128)$ & & $\textit{h}_{ln}^{a}~(128)$ & & Layer Normalization \cite{ba2016layer} \\
\textit{Fully-connected} & & $\textit{h}_{ln}^{a} \forall a \in \{1,2,...,A\}$ & & $\bm{Q}~(A, 128)$  & & \text{activation}$\coloneqq$\text{Linear} \\
\textit{Fully-connected} & & $\textit{h}_{ln}^{a} \forall a \in \{1,2,...,A\}$ & & $\bm{K}~(A, 128)$ & & \text{activation}$\coloneqq$\text{Linear} \\
\textit{Fully-connected} & & $\textit{h}_{ln}^{a} \forall a \in \{1,2,...,A\}$ & & $\bm{V}$~(A, 128) & & \text{activation}$\coloneqq$\text{Linear} \\
\textit{Attention} & & $Q^{a}, \bm{K}, \bm{V}$ & & $\textit{h}_{\textit{atn}}^{a}~(128)$ & & \text{Scaled dot-product attention} \\
\textit{Addition} & & $h^{a}_{0}, \textit{h}_{\textit{atn}}^{a}$ & & $\tilde{h}^{a}$~(128) & & $\tilde{h}^{a} = h^{a}_{0} +  \textit{h}_{\textit{atn}}^{a}$\\
\hline
\multicolumn{7}{c}{\textsc{Local Scene Extractor}} \\
\multicolumn{7}{c}{$\text{(Repeated for } a \in \{1,2,...,A\})$} \\
\hline
\textit{Bilinear} & & $\bm{\Gamma}_l, \hat{S}^{a}_{t-1}~(2)$ & & $\gamma^{a}_{t}$~(6) & & \text{$2\times2$ Bilinear Interpolation}\\
\textit{Concatenate} & & $\tilde{h}^{a}, \gamma^{a}_{t}$ & & $\textit{hg}^{a}_{t}~(134)$ & & \text{-} \\
\textit{Fully-connected} & & $\textit{hg}^{a}_{t}$ & & $f\textit{hg}^{a}_{t}~(50)$ & & \text{activation}$\coloneqq$\text{Softplus} \\
\textit{Fully-connected} & & $f\textit{hg}^{a}_{t}$ & & $\textit{lc}^{a}_{t}~(50)$ & & \text{activation}$\coloneqq$\text{Softplus}\\
\hline
\multicolumn{7}{c}{\textsc{Agent-to-scene Interaction Module}} \\
\multicolumn{7}{c}{$\text{(Repeated for } a \in \{1,2,...,A\} \text{ with the fixed decoding time length } 6)$} \\
\hline
\textit{Flatten} & & $\hat{S}^{a}_{0:t-1}~(t,2)$ & & $\textit{f}\hat{S}^{a}_{0:t-1}~(12)$ & & \text{zero-pad (at the last), }$\hat{S}^{a}_{0} \coloneqq {S}^{a}_{0}$ \\
\textit{GRU} & & $\textit{f}\hat{S}^{a}_{0:t-1}$ & & $\hat{h}^{a}_{t}$ (150) & & \text{zero initial state} \\
\textit{Fully-connected} & & $\hat{h}^{a}_{t}$ & & $\textit{fh}^{a}_{t}$ (150) & & \text{activation}$\coloneqq$\text{Linear} \\
\textit{Fully-connected} & & $\bm{\Gamma}_{g}$ & & $\textit{f}\bm{\Gamma}$ (32, 32, 150) & & \text{activation}$\coloneqq$\text{Linear} \\
\textit{Attention} & & $\textit{fh}^{a}_{t}, \textit{f}\bm{\Gamma}$ & & $\alpha\bm{\Gamma}^{a}_{t}$ (32, 32, 1) & & \text{Additive attention} \\
\textit{Pool} & & $\bm{\Gamma}_{g}, \alpha\bm{\Gamma}^{a}_{t}$ & & $\tilde{\gamma}^{a}_{t}$ (32) & & $\text{Pixel-wise sum }(\bm{\Gamma}_{g} \odot \alpha\bm{\Gamma}^{a}_{t})$ \\
\textit{Concatenate} & & $\tilde{\gamma}^{a}_{t}, \hat{h}^{a}_{t}, \textit{lc}^{a}_{t}$ & & $\textit{gc}^{a}_{t}$ (232) & & \text{-} \\
\hline
\multicolumn{7}{c}{\textsc{Flow Decoder}} \\
\multicolumn{7}{c}{$\text{(Repeated for } a \in \{1,2,...,A\})$} \\
\hline
\textit{Fully-connected} & & $\textit{gc}^{a}_{t}$ & & $\textit{f}{gc}^{a}_{t}$ (50) & & \text{activation}$\coloneqq$\text{Softplus} \\
\textit{Fully-connected} & & $\textit{f}{gc}^{a}_{t}$ & & $\textit{ff}{gc}^{a}_{t}$ (50) & & \text{activation}$\coloneqq$\text{Tanh} \\
\textit{Fully-connected} & & $\textit{ff}{gc}^{a}_{t}$ & & $  \hat{u}^{a}_{t}~(2), \hat{\sigma}^{a}_{t}~(2,2)$ & & \text{activation}$\coloneqq$\text{Linear} \\
\textit{Expm} & & $\hat{\sigma}^{a}_{t}$ & & ${\sigma}^{a}_{t}~(2,2)$ & & impl. in \cite{bernstein1993some} \\
\textit{Constraint} & &
$\hat{\mu}^{a}_{t}, \hat{S}^{a}_{t-2:t-1}$
& &
$\mu^{a}_{t} (2)$
& &
$\alpha\coloneqq0.5$ \\
\textit{Random.} & &
\text{-}
& &
$z^{a}_{t} (2)$
& &
$z^{a}_{t} \sim \mathcal{N}(0, I)$ \\
\textit{Transform} & &
$z^{a}_{t}, \mu^{a}_{t}, \sigma^{a}_{t}$
& &
$S^{a}_{t} (2)$
& &
$S^{a}_{t} = \sigma^{a}_{t} z^{a}_{t} + \mu^{a}_{t}$ \\
\hline
\end{tabular}
\end{center}
\label{tab:parameters}
\end{table*}

%\section{Results Visualisation}

% CAN MOVE VIZ RESULTS HERE

%A notable benefit of our factorising the urban driving problem---into encoding, distribution-aware goal prediction, conformant model-based planning, and pruning + action-selection---is that we obtain increased interpretability in our agent's prediction pipeline. Specifically, by way of our goal-prediction module, we obtain the ability to reveal agent intentionality, during its simulated task execution. Figure \ref{ad:l2d:fig:frames} offers qualitative results from our agent's interaction with the environment, during inference on a randomly-sampled episode. Each frame captures the agent's prediction (in red), given its own speed information, ego-vision context, and short waypoint sequences (in mustard). We observed that waypoint sequences, provided by the environment, may sometimes change, as agents approach locations where some decision must be made (e.g., turns). Coupled with our models estimation of the underlying action distribution, conditioned on offline dataset samples, our model correctly makes multiple admissible predictions of turning (a), going straight (b), changing lanes (c), or stopping/slowing (d) as it approaches the first intersection. After committing and executing the turn (e-f), the agent once again considers multiple possible futures (g), before once again following the rightward arcing waypoint sequence. On straight sections, the agent shows strong belief on forward movement, indicated by distant and straight goal predictions (h), but correctly slows (i) and stops (j) for obstacles.
